# Supplementary material for: Solving Discounted Stochastic Two-Player Games with Near-Optimal Time and Sample Complexity
Source: arXiv:1908.11071 source file (2019-08-29)
Supplement: Supplementary file 1 [file appendix.tex]

\section*{Appendix}
%\mw{Some proof moved here}
We note the following properties of the flux ratio and the ergodicity ratio. Their values are very close to each other when $\gamma\approx 1$.

\begin{lemma}
If a game is ergodic with some constants $0<c_{\min}\le c_{\max}$, then there exists some constants $0<\delta_{\min}\le \delta_{\max}$,
\[
\forall \sigma:\quad \delta_{\min}\cdot\one \le \bx^{\sigma} \le \delta_{\max}\cdot\one.
\]
Moreover
\[
\frac{1}{1-\gamma}\cdot \frac{c_{\min}}{c_{\max}}\le \delta_{\min}\le \delta_{\max} \le \frac{1}{1-\gamma}\cdot \frac{c_{\max}}{c_{\min}}.
\]

\end{lemma}
\begin{proof}
We show the upper bound and the lower bound follows similarly.
\begin{align*}
\bx^\sigma = \sum_{t=0}^\infty \gamma^t (\bP_{\sigma}^{\top})^{t} \one \le \sum_{t=0}^\infty \gamma^t (\bP_{\sigma}^{\top})^{t} \frac{\blambda^{\sigma}}{c_{\min}}
\le \sum_{t=0}^\infty  \frac{\gamma^t \blambda^{\sigma}}{c_{\min}}
\le \sum_{t=0}^\infty  \frac{\gamma^t c_{\max}}{c_{\min}}
 =\frac{1}{1-\gamma}\cdot \frac{c_{\max}}{c_{\min}}.
\end{align*}
%\mw{Move its proof to supp.}
\end{proof}
From the definition, we notice that the flux vector and the eigenvector of a strategy probability share very similar structure.
In fact, we can show the following property.
\begin{lemma}
\begin{align*}
\lim_{\gamma\rightarrow 1} \frac{\delta_{\max}}{\delta_{\min}}
 = \frac{c_{\max}}{c_{\min}}
\end{align*}
%\mw{We probably dont need an epsilon-delta argument here. We can simply say delta is continuous wrt gamma by the definition and invertibility of $1-P$ .. Let's move its proof to supp.}
\end{lemma}
\begin{proof}
Since $\lambda^{\sigma} = \lim_{t\rightarrow\infty}(t)^{-1}\sum_{i=0}^{t-1} (\bP_{\sigma}^\top)^i \one$, %\textcolor{red}{Check}, 
then for any $\epsilon >0$ there exists $T \ge 0$ such that
\[
\forall t\ge T: \qquad\bigg\|\sum_{i=0}^{t-1}(\bP_{\sigma}^\top)^i \one  - t\blambda^{\sigma}\bigg\|_{\infty} \le t\epsilon.
\]
We now consider a fixed $\epsilon<1$, and let $\gamma \ge 1-\epsilon/T$, then we have $\gamma^{T-1} \ge 1 - 2\epsilon$.
We thus obtain,
\begin{align*}
\bx^{\sigma} = \sum_{t=0}^{\infty}  (\gamma \bP_{\sigma}^{\top})^t \one
&=  
\sum_{j=0}^{\infty} \gamma^{jT}(\bP_{\sigma}^{\top})^{jT}\sum_{i=0}^{T-1} \gamma^i(\bP_{\sigma}^{\top})^i \one\\
&\ge \sum_{j=0}^{\infty} \gamma^{jT}(\bP_{\sigma}^{\top})^{jT}\sum_{i=0}^{T-1} (1-2\epsilon)(\bP_{\sigma}^{\top})^i \one\\
&\ge \sum_{j=0}^{\infty} \gamma^{jT}(\bP_{\sigma}^{\top})^{jT}
(1-2\epsilon) T(\blambda^{\sigma} - \epsilon\one)\\
&\ge \sum_{j=0}^{\infty} \gamma^{jT}(\bP_{\sigma}^{\top})^{jT}\cdot
(1-2\epsilon)\cdot T\cdot(1- \epsilon/c_{\min})\cdot \blambda^{\sigma}\\
%&\ge \frac{T(1-2\epsilon)}{1-\gamma^T}(\lambda^{\sigma}) - \\
&\ge T\cdot \frac{\gamma^{T}}{1-\gamma^T}\cdot (1-2\epsilon)(1- \epsilon/c_{\min})\cdot c_{\min}
%\sum_{t=0}^{T}  \gamma^t(P_{\sigma}^{\top})^t \one
% + \sum_{t=T+1}^{\infty}  \gamma^t(P_{\sigma}^{\top})^t \one\\
%&=\sum_{t=0}^{T}  \gamma^t(P_{\sigma}^{\top})^t \one
%+ \sum_{t=T+1}^{\infty}  \gamma^t (\lambda^{\sigma} + \xi_t)
\end{align*}
%where $\xi_t = (P_{\sigma}^{\top})^t \one - \lambda^{\sigma}$ with $\|\xi_t\|_{\infty}\le \epsilon$.
On the other hand, we immediately have
\[
\bx^{\sigma} \le  \sum_{j=0}^{\infty} \gamma^{jT}(\bP_{\sigma}^{\top})^{jT} T(\blambda^{\sigma} + \epsilon\one)
\le \frac{T\gamma^{T}}{1-\gamma^T}(1 +\epsilon/c_{\min})\blambda^{\sigma}
 \le \frac{T\gamma^{T}}{1-\gamma^T}(1 +\epsilon/c_{\min}) \cdot c_{\max}
\]
%Therefore, we have
%\[
%x^{\sigma} \le T +  \frac{\gamma^{T+1}}{1-\gamma}\cdot \lambda^{\sigma} + \frac{\gamma^{T+1}\cdot \epsilon}{1-\gamma}
%\quad\text{and}\quad
%x^{\sigma} \ge   \frac{\gamma^{T+1}}{1-\gamma}\cdot \lambda^{\sigma} - \frac{\gamma^{T+1}\cdot \epsilon}{1-\gamma}.
%\]
Hence we obtain,
\[
\frac{c_{\max}}{c_{\min}}= \frac{\delta_{\max}}{\delta_{\min}}
\cdot(1\pm 3\epsilon \pm 3\epsilon/c_{\min})
\]
for sufficiently small $\epsilon$.
Consider $\epsilon =  \epsilon'c_{\min}$ for some sufficient small $\epsilon'< 1$.
We have
\[
 3\epsilon + 3\epsilon/c_{\min}
\le 6\epsilon'.
\]
%
%Consider $\gamma = 1 - \epsilon^2/T$, 
%we then have $\gamma^{T+1} \ge 1/2$ for sufficiently small $\epsilon$ and
%\[
%x^{\sigma} \le 
%c_{\max} \cdot \frac{\gamma^{T+1}}{1-\gamma^T}
%+ \frac{\gamma^{T+1}}{1-\gamma^T}\cdot (\epsilon + 2\epsilon^2)
%\quad\text{and}\quad
%x^{\sigma} \ge 
%c_{\min} \cdot \frac{\gamma^{T+1}}{1-\gamma^T}
%- \frac{\gamma^{T+1}}{1-\gamma^T}\cdot \epsilon.
%\]
%Suppose $\epsilon\le \epsilon'\cdot c_{\min} \ll 1$ for some small $\epsilon'$, we have
%\[
%x^{\sigma}\le (1+3\epsilon')\cdot c_{\max} \cdot \frac{\gamma^{T+1}}{1-\gamma^T}
%\quad\text{and}\quad 
%x^{\sigma}\ge (1-\epsilon'/2)\cdot {c_{\min}} \cdot \frac{\gamma^{T+1}}{1-\gamma^T}.
%\]
%Eventually, we have,
%\[
%\frac{c_{\max}}{c_{\min}}\le \frac{\delta_{\max}}{\delta_{\min}}
%\le \frac{c_{\max}}{c_{\min}}+ 4\epsilon'.
%\]
Since for any sufficiently small $\epsilon'$, there is always a $T$, hence a $\gamma$, s.t. the above formula holds, we conclude the proof.
\end{proof}
